# Supplementary material for: SYNC-CLIP: Synthetic Data Make CLIP Generalize Better in Data-Limited Scenarios
Source: arXiv:2312.03805 source file (2023-12-06)
Supplement: Supplementary file 1 [file main_appendix.tex]

% CVPR 2024 Paper Template; see https://github.com/cvpr-org/author-kit
\documentclass[10pt,twocolumn,letterpaper]{article}
%%%%%%%%% PAPER TYPE  - PLEASE UPDATE FOR FINAL VERSION
% \usepackage{cvpr}              % To produce the CAMERA-READY version
\usepackage[review]{cvpr}      % To produce the REVIEW version
\usepackage{graphicx}
\usepackage{amssymb}
\usepackage{booktabs}
\usepackage{multirow}
\usepackage{amsmath}
\usepackage{subcaption}
\usepackage{tablefootnote}
\usepackage[dvipsnames]{xcolor}

\usepackage{amsmath}
\usepackage{tabularx} % 用于自动调整列宽
\usepackage{booktabs}
\usepackage{tikz}
\usepackage{xcolor}         % colors
\usepackage{colortbl}
\usepackage{rotating}

\usepackage{bbding}
\usepackage{multirow}
\usepackage{xcolor}         % colors
\usepackage{colortbl}
\usepackage{overpic}
\usepackage{indentfirst} 
\usepackage{graphicx}

\usetikzlibrary{tikzmark, positioning, arrows.meta}
% \usepackage[pagenumbers]{cvpr} % To force page numbers, e.g. for an arXiv version
% Import additional packages in the preamble file, before hyperref
\input{preamble}
% It is strongly recommended to use hyperref, especially for the review version.
% hyperref with option pagebackref eases the reviewers' job.
% Please disable hyperref *only* if you encounter grave issues, 
% e.g. with the file validation for the camera-ready version.
%
% If you comment hyperref and then uncomment it, you should delete *.aux before re-running LaTeX.
% (Or just hit 'q' on the first LaTeX run, let it finish, and you should be clear).
\definecolor{cvprblue}{rgb}{0.21,0.49,0.74}
\usepackage[pagebackref,breaklinks,colorlinks,citecolor=cvprblue]{hyperref}
\usepackage[capitalize]{cleveref}
\crefname{section}{Sec.}{Secs.}
\Crefname{section}{Section}{Sections}
\Crefname{table}{Table}{Tables}
\crefname{table}{Tab.}{Tabs.}

%%%%%%%%% PAPER ID  - PLEASE UPDATE
 % *** Enter the Paper ID here

%%%%%%%%% TITLE - PLEASE UPDATE
% \title{Synthetic Data Make Strong Visual Learners for Data-Limited Scenarios} % xx are strong visual learners
% \title{Synthetic Data Make Visual Learners Stronger for Data-Limited Scenarios}
\title{SYNC-CLIP: Synthetic Data Make CLIP Generalize Better in\\
Data-Limited Scenarios}

%%%%%%%%% AUTHORS - PLEASE UPDATE
\author{First Author\\
Institution1\\
Institution1 address\\
{\tt\small firstauthor@i1.org}
% For a paper whose authors are all at the same institution,
% omit the following lines up until the closing ``}''.
% Additional authors and addresses can be added with ``\and'',
% just like the second author.
% To save space, use either the email address or home page, not both
\and
Second Author\\
Institution2\\
First line of institution2 address\\
{\tt\small secondauthor@i2.org}
}

\begin{document}
\definecolor{lightblue}{rgb}{0.93,0.95,1.0}
\definecolor{mediumblue}{rgb}{0.0,0.45,0.73}

% \maketitle
% \input{sections/abstract}
% \input{sections/introduction}
% \input{sections/related_works}
% \input{sections/methodology}
% \input{sections/experiments}
% \input{sections/conclusion}
% \newpage

% % WARNING: do not forget to delete the supplementary pages from your submission 
% \newpage
% \newpage
\input{sections/appendix}
{
    \small
    \bibliographystyle{ieeenat_fullname}
    \bibliography{main}
}
\end{document}
